# Supplementary material for: Modeling Intensification for Sign Language Generation: A Computational Approach
Source: arXiv:2203.09679 source file (2022-03-18)
Supplement: Supplementary file 1 [file appendix_result_tables.tex]

\begin{table*}[b!]
\small
    \centering
    \setlength\tabcolsep{3.5pt}
    \begin{tabular}{c|ccccc|ccccc}
    \toprule
        & \multicolumn{5}{|c}{DEV SET} & \multicolumn{5}{|c}{TEST SET} \\
        \midrule
        Model & BLEU-1 & BLEU-2 & BLEU-3 & BLEU-4 & ROUGE & BLEU-1 & BLEU-2 & BLEU-3 & BLEU-4 & ROUGE \\

         \midrule
         
         G2S &  29.92 & 20.00 & 14.94 & 11.90 & 30.05 & 29.86 & 19.93 & 14.63 & 11.51 & 29.13 \\ 
         TG2S &  29.02 & 19.45 & 14.49 & 11.57 & 29.56 & 29.42 & 20.03 & 14.83 & 11.63 & 29.61\\

        %  BETWEEN & 31.22 & 21.28 & 15.93 & 12.54 & 31.57 & 29.38 & 20.04 & 14.94 & 11.98 &  30.24 \\
        % %  BETWEENRepeat & 30.06 & 19.84 & 14.64 & 11.59 & 30.15 & 29.48 & 19.71 & 14.33 & 11.11 & 29.26 \\
        %  BEFORE & 32.03 & 21.52 & 15.82 & 12.36 & 31.75 & 27.08 & 18.05 & 13.10 & 10.27 & 26.61 \\
        % %  JOINT & 31.23 & 21.30 & 15.96 & 12.56 & 31.58 & 29.15 & 19.41 & 14.11 & 11.05 & 28.87 \\
        % %  JOINT-Repeat & 30.60 & 20.49 & 15.09 & 11.83 & 31.02 & 29.90 & 20.01 & 14.68 & 11.63 & 29.87\\
        % % BETWEEN & 22.54 & 13.84 & 9.74 & 7.46 & 23.13 & 20.63 & 12.79 & 8.94 & 6.89 & 21.39\\
        % % BETWEEN\_repeat & 23.15 & 14.81 & 10.64 & 8.29 & 23.30 & 23.21 & 14.72 & 10.43 & 8.01 & 23.24 \\
        % % JOINT &  & \textbf{4.21} & \textbf{12.96} \\
        % % BEFORE & 12.50 & 6.80 & 4.78 & 3.71 & 12.46 \\
        \hline
    \end{tabular}
    \caption{Back translation results obtained from the different generative models wh We use Carla's best ckpt as the BT model for Baseline, and all others with retrained BT model in correspondence to the augmented gloss. For BETWEENRepeat, since the SLT model give bad performance, we used the SLT trained on BETWEEN instead.}
    \label{tab:models}
\end{table*}
